# Supplementary material for: On identifying dynamic length scales in crystal plasticity
Source: arXiv:2406.09892 source file (2024-06-14)
Supplement: Supplementary file 1 [file sm.pdf]

# Supplementary Materials for “On identifying dynamic length scales in crystal plasticity”

Dénes Berta<sup>a</sup>, David Kurunczi-Papp<sup>b</sup>, Lasse Laurson<sup>b,\*</sup>, Péter Dusán Ispánovity<sup>a,\*</sup>

<sup>a</sup>*Department of Materials Physics, ELTE Eötvös Loránd University, Pázmány Péter sétány 1/a, 1117 Budapest, Hungary*

<sup>b</sup>*Computational Physics Laboratory, Tampere University, P.O. Box 692, FI-33014 Tampere, Finland*

---

## 1. Avalanche detection threshold

The noise level and the typical size of plastic strain rate bursts being dependent on the box size, different plastic strain rate thresholds were applied to detect avalanches. The thresholds are summarized in Tab. 1.

| threshold                        | no precipitates | precipitates |
|----------------------------------|-----------------|--------------|
| $\dot{\varepsilon}_{p,th}^{(0)}$ | 1700            | 1700         |
| $\dot{\varepsilon}_{p,th}^{(1)}$ | 1700            | 1700         |
| $\dot{\varepsilon}_{p,th}^{(2)}$ | 9500            | 9500         |

Table 1: Plastic strain rate thresholds utilized for avalanche detection.  $\dot{\varepsilon}_p^{(b)}$  denotes the plastic strain rate at box division level  $B = b$ .

## 2. Local yield stress tree charts

The tree charts representing the local yield stresses for all scales ( $B = 0, 1, 2$ ) are shown for all individual configuration in Figs. 1 and 2. The arrows point from the weakest subbox to its parent box the black arrows indicating that the inheritance of local yield stress is satisfied (with less than a factor of 2 difference between the local yield threshold of the subbox and the parent box). If this criterion is not met, it is signified by a red arrow. This inheritance criterion is satisfied half of the time (49%) and with a probability of c. 3/4 (73%) in the case of configurations without and with precipitates, respectively.

## 3. Identification of dislocation lines

In order to execute some of the analysis in the main paper, it has to be distinguished whether two dislocation nodes are from the same or different dislocation lines. We considered two nodes to be of the same dislocation if one node can be reached from another through dislocation segments while avoiding dislocation junctions. The representation of the distinct dislocation lines is shown in Fig. 3 for a representative configuration.

---

\*Corresponding authors

Email addresses: `lasse.laurson@tuni.fi` (Lasse Laurson), `ispanovity.peter@ttk.elte.hu` (Péter Dusán Ispánovity)

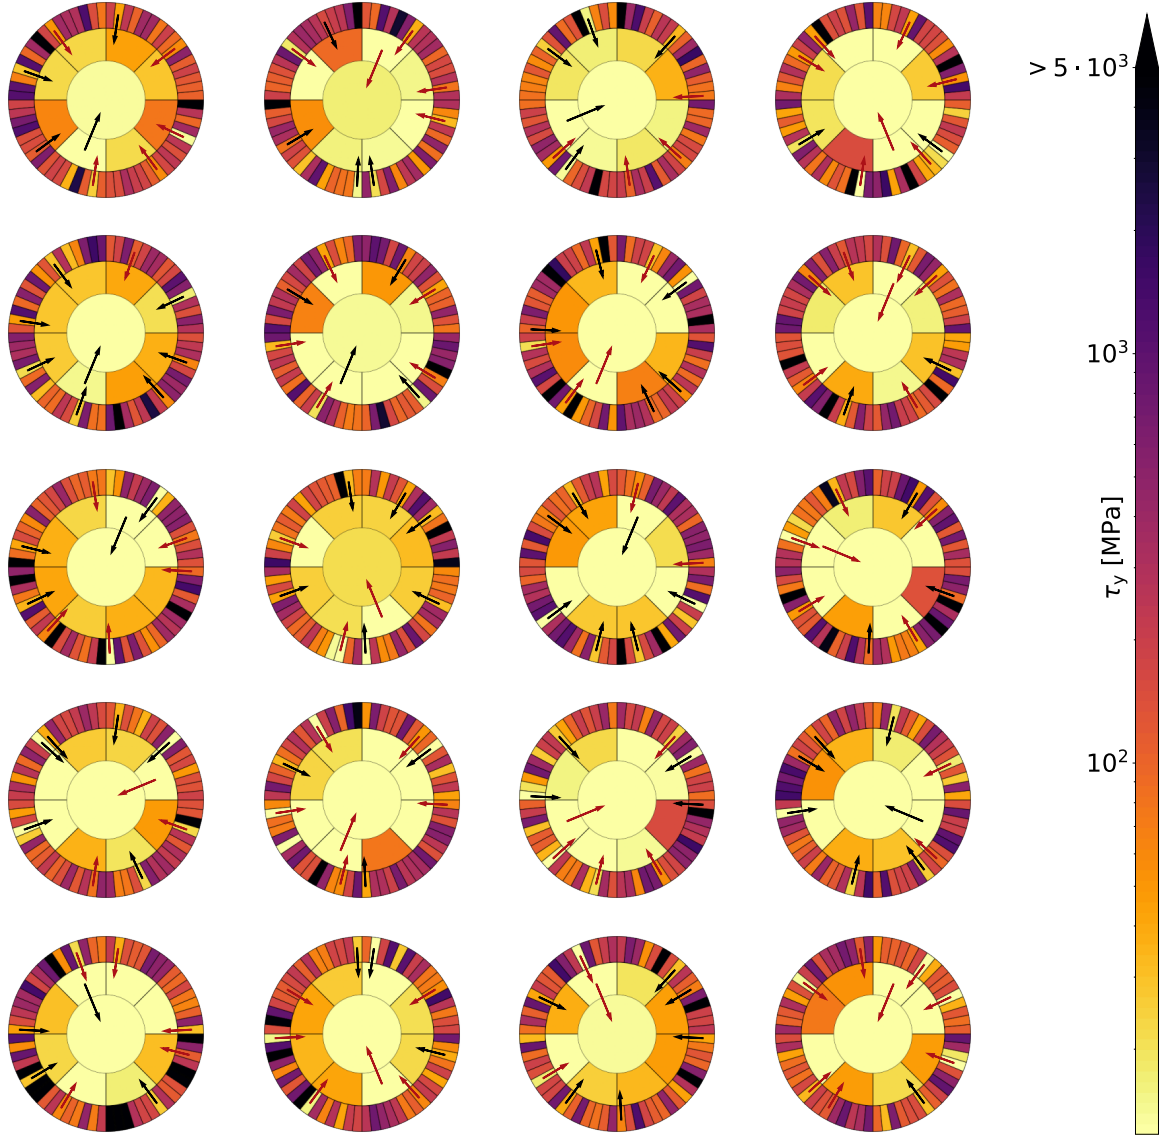

Figure 1: Local yield stress tree charts of configurations without precipitates. The black arrows signify that the local yield stress is inherited from the softest subbox (with an error up to a factor of two) while red arrows indicate the violation of this inheritance.

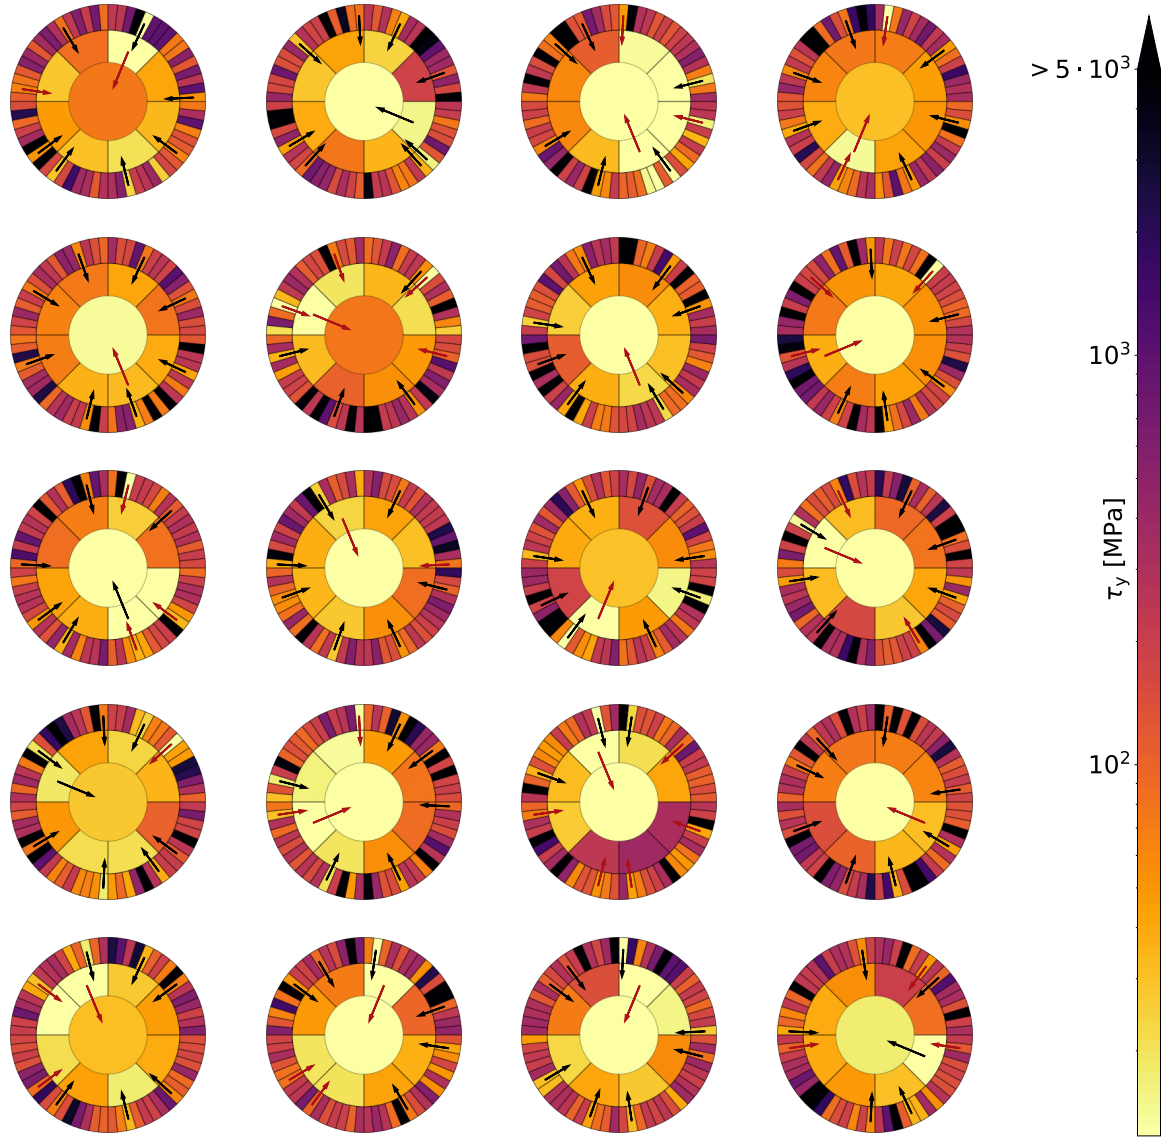

Figure 2: Local yield stress tree charts of configurations with precipitates. The black arrows signify that the local yield stress is inherited from the softest subbox (with an error up to a factor of two) while red arrows indicate the violation of this inheritance.

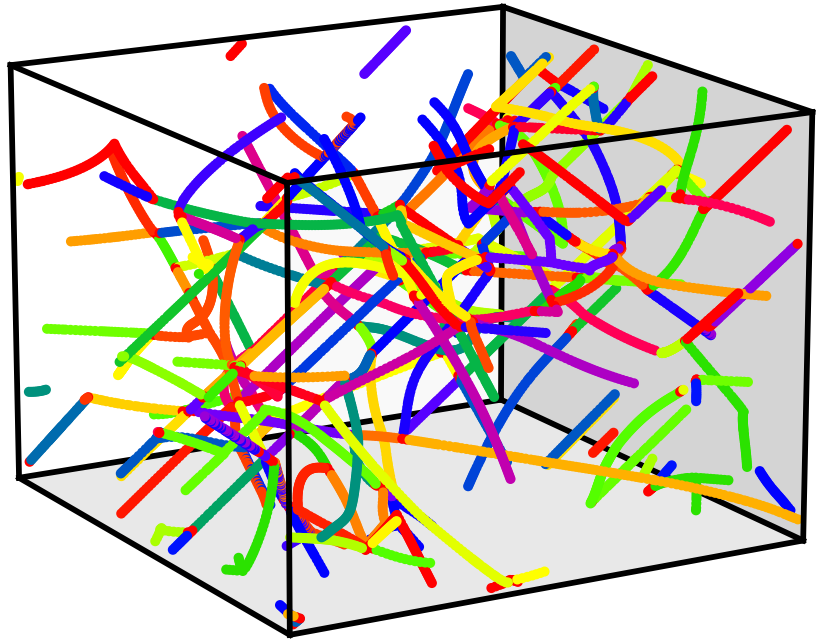

Figure 3: A representative configuration showing distinct dislocation lines in different colors. Note that due to the large number of lines a few different dislocation lines might appear in very similar colors.
